# Supplementary material for: Memory Under Siege: A Comprehensive Survey of Side-Channel Attacks on Memory
Source: arXiv:2505.04896 source file (2025-05-08)
Supplement: Supplementary file 1 [file appendix.tex]

\appendix 
==========================
\section{Software-Based Attacks}
The software layer, while enabling flexibility and performance, often harbors subtle vulnerabilities that attackers can exploit. Software-based side-channel attacks target these vulnerabilities, leveraging flaws in program logic, memory management, and microarchitectural design to extract sensitive data or disrupt system operations. These attacks exploit unintended behaviors that arise from optimizations meant to improve efficiency, revealing the intricate interplay between software and hardware in modern computing systems. Among the most studied categories are speculative and transient execution attacks, which exploit processor mechanisms like branch prediction and out-of-order execution. These attacks, exemplified by Spectre and Meltdown, have reshaped the understanding of hardware vulnerabilities by exposing the risks inherent in speculative optimizations \cite{kocher2020spectre, lipp2020meltdown}. Beyond speculative execution, software-based attacks include memory and page table manipulation, where techniques such as Rowhammer \cite{kim2014flipping} or page table exploit target memory operations to breach isolation \cite{van2017telling}. Furthermore, secure enclave exploitation highlights vulnerabilities in trusted execution environments like Intel SGX\cite{chen2019sgxpectre}, while timing-based attacks leverage discrepancies in execution time to infer sensitive information\cite{zhou2016software, }. Finally, shared library and API exploitation demonstrates how predictable patterns in shared resources can inadvertently create side channels \cite{gruss2015cache}.
In the following sections, we systematically explore these attack types, starting with speculative and transient execution, followed by other prominent categories. This progression offers a comprehensive view of the diverse methodologies that define software-based side-channel attacks.

\subsection{Transient and Speculative Execution Attacks}
In the relentless pursuit of speed, modern processors have adopted speculative execution—a technique that anticipates program behavior to execute instructions ahead of time. This innovation has revolutionized computing performance, enabling processors to stay a step ahead of user instructions. However, this speculative ability comes with a cost: the transient states created during speculation are not fully isolated, and these fleeting moments of vulnerability have become a gold mine for attackers.
The story of transient execution attacks begins with Spectre and Meltdown, two groundbreaking discoveries that turned the computing world on its head \cite{kocher2020spectre, lipp2020meltdown}. These attacks revealed that speculative execution, once seen solely as a performance optimization, could be manipulated to leak sensitive data across even the most secure boundaries. The discoveries ignited a wave of research, each step revealing deeper layers of vulnerability within the speculative machinery of processors.

\begin{itemize}
    \item \textbf{Branch Prediction Attack:}
    At the heart of speculative execution lies branch prediction—a mechanism that enables processors to "guess" the outcome of a conditional branch. By anticipating the likely path of execution, processors avoid wasting cycles while waiting for the branch to resolve. However, what happens when the guess is wrong? Attackers realized that these mispredictions create transient states that can be exploited to access sensitive data \cite{evtyushkin2018branchscope} \cite{mcilroy2019spectre}. The first strike came with Spectre v1, a proof of concept that demonstrated how attackers could mistrain branch predictors to force processors down an invalid path. This "bounds check bypass" attack accessed out-of-bounds memory during speculation, leaving traces in the cache that attackers could analyze to infer data \cite{kocher2020spectre}. Building on this foundation, Spectre v2 turned its attention to indirect branch prediction. Here, attackers injected malicious branch targets into the predictor, redirecting speculative execution toward attacker-controlled instructions. The implications were staggering: sensitive data could be leaked from privileged processes, and even cloud environments could no longer ensure tenant isolation.As researchers peeled back the layers of speculative execution, more avenues for exploitation emerged. SpectreRSB demonstrated how the return stack buffer—responsible for predicting return addresses—could be manipulated to hijack speculative execution paths\cite{koruyeh2018spectre}. Similarly, Spectre-PHT targeted pattern history tables, exposing the vulnerabilities in branch prediction’s historical tracking mechanisms\cite{chowdhuryy2021leaking}. Together, these discoveries painted a grim picture: speculative execution was not just a performance tool but a doorway to systemic exploitation.

    \item \textbf{Instruction-Level Attacks:}
    Instruction-level side-channel attacks delve into the fine-grained behaviors of speculative execution, focusing on how even isolated instructions can create exploitable side channels. These attacks target specific instructions, leveraging their transient effects to uncover sensitive data patterns. Flush+Flush, for instance, bypasses the need for shared memory by measuring timing differences in cache flush operations to detect cache residency \cite{gruss2016flush+}. Unlike its predecessor Flush+Reload, which requires memory sharing \cite{yarom2014flush+}, Flush+Flush leverages timing precision, enabling attackers to extract sensitive information \cite{gruss2016prefetch}. Another critical example is Speculative Store Bypass (SSB), which demonstrates how stale values can be forwarded between speculative store and load operations. This attack reveals critical vulnerabilities in speculative execution paths that propagate unintended data flows\cite{kiriansky2018speculative}.These instruction-level attacks illustrate the vulnerabilities introduced by speculative optimizations, exposing the fragility of modern microarchitectural designs.

    \item \textbf{Out-of-Order Execution:}
     While branch prediction exploits revealed the fragility of speculative control flow, attacks such as Meltdown showed that the problem extended deeper into the processor pipeline. Out-of-order execution, a technique designed to maximize parallelism by executing instructions as soon as their dependencies are resolved, was found to operate on sensitive data during speculation \cite{lipp2020meltdown}. Meltdown showed how speculative memory loads could bypass privilege checks, allowing attackers to read kernel memory from user space. The attack shook the industry, exposing passwords, cryptographic keys, and other sensitive data stored in kernel space. Meltdown proved that speculative execution vulnerabilities were not confined to user-space operations; they could strike at the heart of system security. Following Meltdown, Fallout shifted focus to store buffers, revealing additional speculative vulnerabilities in transient states.\cite{canella2019fallout}.

     \item \textbf{Buffer Exploits:}
     Buffers used in speculative execution, such as store buffers or load ports, represent another avenue for exploitation. These shared microarchitectural resources are designed to enhance processing efficiency but inadvertently become channels for transient data leakage. RIDL (Rogue In-Flight Data Load), for instance, targets load ports to extract transient data, showcasing how critical information can be accessed during speculative execution paths\cite{van2019ridl}. Attacks like ZombieLoad and CrossTalk further demonstrate the risks posed by shared buffers. ZombieLoad exploits fill buffers to leak information processed by other threads, highlighting vulnerabilities in cross-thread isolation \cite{schwarz2019zombieload}. Meanwhile, CrossTalk shows how shared buffers can enable data leakage across CPU cores, underscoring the systemic risks inherent in shared microarchitectural resources\cite{ragab2021crosstalk}. These buffer exploits underline the unintended consequences of speculative execution optimizations, emphasizing the need for more robust resource isolation in future processor designs.

     \item \textbf{Cache-Based Attacks:} 
     Caches, the high-speed memory designed to bridge the gap between processors and main memory, are another cornerstone of speculative execution. While crucial for performance, caches also became silent witnesses to speculative operations, revealing their secrets through timing differences. The journey into cache-based side channels began with Flush+Reload, a technique that exploited shared memory to infer cache line residency\cite{yarom2014flush+}. By evicting a cache line and measuring the time taken for the victim to reload it, attackers could determine whether the victim accessed the data. This method became a blueprint for future cache attacks, particularly in cryptographic settings\cite{gruss2015cache, kocher2020spectr}. Prime+Probe soon followed, eliminating the need for shared memory by filling cache sets with attacker-controlled data and monitoring eviction patterns caused by victim activity \cite{gruss2015cache, younis2015new, kocher2020spectre}. This attack proved especially potent in cloud environments, where shared resources were abundant, but direct memory sharing was restricted. The sophistication of cache-based attacks reached new heights with ZombieLoad, which targeted fill buffers to leak data processed by other threads\cite{schwarz2019zombieload}. ZombieLoad revealed that even processes operating in isolation could be compromised through shared microarchitectural components. CacheOut, meanwhile, refined the art of cache exploitation by allowing attackers to selectively target specific data in the L1-D cache, marking a new era of precision in side-channel attacks\cite{van2021cacheout}.
\end{itemize}

\subsection{Secure Enclave Exploitation:}
Secure enclaves, like Intel's Software Guard Extensions (SGX), were introduced as a cornerstone of modern trusted computing. By isolating sensitive computations within protected regions, enclaves promised unparalleled security, even in the presence of compromised operating systems. However, this promise has been repeatedly challenged by sophisticated attacks that exploit microarchitectural flaws, revealing vulnerabilities in these trusted execution environments. From Branch Shadowing to Foreshadow, these attacks expose how performance-optimized features, such as speculative execution and shared resources, can become gateways for adversaries to compromise the integrity of secure enclaves. Each category of these attacks highlights unique vulnerabilities, setting the stage for a deeper exploration of the intricate interplay between secure enclave mechanisms and microarchitectural designs.

\begin{itemize}

    \item \textbf{Control Flow Exploits:}
    Modern processors rely heavily on branch predictors to maintain performance, but these mechanisms have become a double-edged sword, as demonstrated by attacks like Branch Shadowing and BranchScope. Branch Shadowing, for instance, manipulates branch predictors to infer fine-grained control flow inside SGX enclaves. By mistraining the branch predictor, attackers can manipulate speculative execution paths, forcing the processor to execute instructions along incorrect speculative branches  \cite{lee2017inferring}. Similarly, BranchScope builds on these principles by manipulating directional branch predictors to expose enclave operations\cite{evtyushkin2018branchscope}.

    \item \textbf{Operating System-Level Exploits:}

    Beyond control flow vulnerabilities, enclaves face significant risks from their reliance on untrusted operating systems. Controlled-channel attacks exemplify this threat by leveraging an OS’s deterministic control over memory access patterns to infer enclave behavior, which manipulates page fault information or memory access timing to bypass the isolation guarantees of SGX. [\textit{Xu et al.}  demonstrate how deterministic side channels can systematically undermine enclave security\cite{xu2015controlled}.Another OS-level exploit, ret2dir, takes advantage of kernel address redirection to compromise memory access paths\cite{kemerlis2014ret2dir}. Similarly, Translation Leak-aside Buffer (TLBleed) targets translation lookaside buffers managed by the operating system, revealing enclave secrets through timing discrepancies\cite{gras2018translation}.Cache Telepathy, another notable attack, leverages timing discrepancies in shared resources, such as cache lines, managed by the OS to infer sensitive data from SGX enclaves \cite{yan2020cache}. Which arise when multiple processes compete for shared hardware resources. Foreshadow-NG expands on these vulnerabilities by exploiting the L1 Terminal Fault to bypass both enclave and kernel isolation\cite{weisse2018foreshadow}.

    \item \textbf{Transient Execution Attacks on SGX:}
    Transient execution attacks exploit speculative states in processors, where instructions are executed ahead of time to improve performance. Foreshadow is a key example, targeting SGX to access protected memory during speculative operations. By leveraging these transient states, Foreshadow bypasses enclave isolation and exposes sensitive data\cite{van2018foreshadow} SpectreRSB exploits the Return Stack Buffer (RSB), a speculative execution component, by manipulating its entries to create false predictions. This enables attackers to leak sensitive data across processes during speculative execution phases\cite{koruyeh2018spectre}. RIDL (Rogue In-Flight Data Load) targets speculative loads by capturing transient data left in microarchitectural buffers during incomplete operations. These speculative states reveal sensitive information that would otherwise be inaccessible\cite{van2019ridl}. ZombieLoad represents another advancement in speculative data leakage techniques, leveraging fill buffers to extract sensitive data across privilege boundaries. Such advancements in transient execution attacks bridge the gap between speculative states and broader exploitation of shared resources\cite{schwarz2019zombieload}. Another noteworthy attack, CopyCat, manipulates instruction-level behaviors to exploit speculative execution paths. By carefully targeting specific execution flows, CopyCat reveals how transient states can be harnessed to leak enclave-protected information \cite{moghimi2020copycat}. SgxPectre adapts Spectre vulnerabilities specifically for SGX enclaves, targeting speculative execution paths to leak sensitive enclave data. This attack exemplifies the challenges in securing speculative execution within trusted environments \cite{chen2019sgxpectre}.

    \item \textbf{Fault Injection Attacks:}
    Fault injection attacks exploit hardware-level vulnerabilities to introduce intentional errors into the computation processes of secure enclaves, disrupting their normal functionality. Plundervolt, for instance, uses software-induced undervolting to induce faults within SGX, enabling unauthorized data access \cite{murdock2020plundervolt}.SmashEx manipulates the OS-enclave interface to exploit exception handling in SGX. By introducing re-entrancy vulnerabilities, SmashEx compromises enclave integrity, highlighting the importance of secure exception handling\cite{cui2021smashex}. SIGY targets the enclave programming model by delivering fake hardware events, corrupting the enclave state and violating execution integrity across multiple runtimes and languages\cite{sridhara2024sigy}. TeeRex uncovers memory corruption vulnerabilities in the host-to-enclave boundary. By exploiting these issues, attackers can corrupt function pointers and perform arbitrary memory writes, undermining enclave security\cite{cloosters2020teerex}.
\end{itemize}

\subsection{Timing-Based Exploitation:}
Timing-based exploitation represents a subtle yet powerful class of side-channel attacks that leverage differences in execution time to infer sensitive information. These attacks exploit timing variations inherent in hardware and software operations, revealing critical details about the system’s behavior. The success of these attacks often hinges on the attacker’s ability to measure execution time with extreme precision, demonstrating the intricate interplay between performance optimization and security vulnerabilities.
\begin{itemize}
    \item \textbf{Cryptographic Timing Attacks:}
    Cryptographic systems, designed to secure sensitive data, are vulnerable to timing-based attacks. These attacks exploit variations in execution time during cryptographic operations to extract secret keys or compromise encryption protocols. A prominent example is the timing attack on RSA implementations, where timing variations in modular exponentiation can reveal private keys \cite{kocher1996timing}.Cache timing attacks are another significant threat, exploiting differences in data access times in cache memory to deduce sensitive information during encryption operations. Access-driven attacks, such as those described in Cache Games—Bringing Access-Based Cache Attacks on AES to Practice, demonstrate how cache behavior can systematically be exploited to break AES encryption in practice \cite{gullasch2011cache}. Efficient cache timing attacks on AES, as discussed by Bernstein, further illustrate the precision with which sensitive information can be extracted, underscoring the need for robust countermeasures \cite{bernstein2005efficient}. Tromer et al. explored how shared cache access in multi-tenant systems can enable timing attacks on AES in virtualization environments, exposing vulnerabilities unique to such setups \cite{tromer2009virtualization}. Furthermore, tools like CacheD provide a framework for identifying cache-based timing channels in production environments, bridging the gap between theoretical attacks and practical implementations \cite{wang2017cached}. Building on these techniques, CacheBleed leverages cache-bank conflicts to target cryptographic processes such as RSA, enabling precise extraction of sensitive information \cite{yarom2017cachebleed}. Additionally, MemJam exploits false dependencies in memory operations, breaking constant-time cryptographic implementations and demonstrating how memory-related software optimizations can inadvertently create exploitable timing channels \cite{moghimi2019memjam}.

    \item \textbf{Application Timing Exploitation:}
    Beyond cryptographic systems, timing-based exploitation extends to application-level behaviors. Attackers leverage predictable execution patterns or timing differences in application workflows to extract sensitive data. For example, timing discrepancies in database queries can reveal information about the underlying data structure or content. Similarly, timing attacks on web servers exploit differences in response times to infer the presence or absence of specific data\cite{felten2000timing}. The Spy in the Sandbox demonstrates how JavaScript-based timing attacks can exploit browser environments to leak sensitive data through the last-level cache\cite{oren2015spy}.Remote Timing Attacks are Practical demonstrates the real-world applicability of timing-based side channels in breaking SSL-enabled web servers. By analyzing subtle variations in encryption processing time, attackers successfully retrieved cryptographic keys, showcasing the broad reach of such exploits\cite{brumley2011remote}.

    \item \textbf{Shared Resource Timing Attacks:}
    Shared resource timing attacks focus on exploiting contention in shared hardware components, such as caches or memory buses. Prime+Probe and Flush+Reload are quintessential examples of such attacks, where attackers manipulate and monitor shared cache lines to infer victim activity. These techniques have been successfully used in cross-VM attacks to extract cryptographic keys from co-resident virtual machines \cite{percival2005cache, yarom2014flush+}. Page Cache Attacks expand on this principle by targeting the operating system’s page cache to create a covert channel for extracting sensitive data\cite{gruss2019page}. DRAMA: Exploiting DRAM Addressing for Cross-CPU Covert Channels demonstrates how timing side channels in DRAM row buffer management can enable covert communication across CPU cores, further emphasizing the systemic risks of shared resource exploitation\cite{pessl2016drama}. Fallout leverages timing discrepancies using Flush+Flush to create cross-core covert channels, showcasing the potential of timing side channels to compromise data even in Meltdown-resistant CPUs\cite{canella2019fallout}. Timeless Timing Attacks explores how concurrency in software systems can be exploited to create timing side channels over remote connections\cite{van2020timeless}.The effectiveness of shared resource timing attacks underscores the challenges of ensuring isolation in multi-tenant environments, particularly in cloud computing scenarios. Fantastic Timers and Where to Find Them highlights how high-resolution timers can be leveraged to amplify timing side channels, further increasing the risk of exploitation\cite{schwarz2017fantastic}.

\end{itemize}

\subsection{Memory and Page Table Manipulation:}
Memory and page table manipulation attacks exploit vulnerabilities in how operating systems and processors manage memory. These attacks take advantage of weaknesses in memory access patterns, cache coherence, or row management to breach isolation boundaries, enabling attackers to tamper with or access sensitive data.
One prominent example is the Rowhammer attack, which exploits hardware-induced bit flips in DRAM memory cells to manipulate adjacent rows of data \cite{mutlu2019rowhammer}. By rapidly activating specific memory rows, attackers induce electromagnetic interference that flips bits in nearby rows. This vulnerability is particularly dangerous because it allows attackers to corrupt data or even escalate privileges without directly accessing the target data\cite{kim2014flipping}.Expanding on Rowhammer, Drammer targets mobile platforms, demonstrating that such attacks are feasible even in constrained environments. Drammer exploits deterministic bit flips to bypass memory isolation mechanisms on ARM-based systems, which underscores the pervasive nature of this threat across different architectures\cite{van2016drammer}.In addition to that, Page Table Exploits manipulate virtual memory mapping to breach isolation boundaries. By exploiting page faults, attackers can infer sensitive data or cause privilege escalation. Techniques like Cross-VM attacks leverage shared memory pages in virtualized environments to extract private data across tenant boundaries. These attacks demonstrate how the interplay between hardware and software can inadvertently create exploitable side channels\cite{zhang2012cross}.

\subsection{Shared Library and API Exploitation:}
Shared libraries and APIs play a crucial role in modern software systems, providing reusable functions and resources for developers. However, the shared and predictable nature of these components often introduces subtle vulnerabilities that attackers can exploit. This section explores how shared libraries and APIs are targeted through side-channel techniques to undermine security features, focusing on Address Space Layout Randomization (ASLR) and memory deduplication.

\begin{itemize}
    \item \textbf{Exploitation Through Shared Libraries:}
    Address Space Layout Randomization (ASLR) is a widely used defense mechanism to randomize the memory layout of programs, making it harder for attackers to predict memory addresses. However, shared libraries and APIs can inadvertently expose predictable behaviors that attackers exploit to bypass ASLR. Jump Over ASLR demonstrates how branch predictors, a shared hardware feature, can be manipulated to bypass ASLR protections. By observing and exploiting branch predictor states, attackers infer memory layout details, revealing sensitive addresses\cite{evtyushkin2016jump}. Similarly, KASLR is Dead: Long Live KASLR targets kernel ASLR by exploiting shared branch predictors. This attack Shows the systemic risk of shared resources in compromising kernel-level randomization, exposing critical kernel memory regions\cite{gruss2017kaslr}. Prefetch Side-Channel Attacks further emphasize the vulnerabilities in shared libraries by exploiting address translation oracles. Attackers leverage prefetch instructions to infer the memory layout of kernel ASLR, creating a novel pathway for bypassing this critical security feature\cite{gruss2016prefetch}. Additionally, Peep With A Mirror explores cache-based side-channel attacks targeting shared libraries on Android systems. This research demonstrates how monitoring shared library functions like libinput.so allows attackers to infer sensitive inputs such as keystrokes, breaking app sandboxing\cite{lin2024peep}. \textit{Irazoqui et al} demonstrates a novel method to exploit shared cache memory, allowing attackers to extract sensitive information across virtual machine boundaries, effectively bypassing VM isolation \cite{irazoqui2015s}.

    \item \textbf{Exploitation Through Shared API:}
    Timing discrepancies in shared APIs can reveal sensitive information about the underlying system. \textit{Hund et al.} demonstrates how timing differences in API responses expose kernel memory layouts. By analyzing response times, attackers infer critical memory locations, bypassing ASLR defenses and compromising kernel-level security\cite{hund2013practical}. Another study, Timing Cache Accesses to Eliminate Side Channels in Shared Software, investigates software designs that mitigate cache-based timing side channels in shared software systems. This work proposes architectural changes to prevent side-channel leaks in shared APIs\cite{ojha2020timing}. \textit{ojha et al.} bypasses traditional cache-based defenses, posing novel challenges for shared library security\cite{ojha2020timing}

    \item \textbf{Memory Deduplication Vulnerabilities:}

    Memory deduplication, a feature used to optimize memory usage in virtualized environments, combines identical memory pages to save space. While beneficial for performance, this mechanism introduces exploitable side channels.The CAIN attack showcases how memory deduplication can be exploited to bypass ASLR in cloud environments. By introducing controlled memory patterns and observing deduplication behavior, attackers infer the memory layout of co-resident virtual machines, silently breaking ASLR protections\cite{barresi2015cain}. \textit{Lindemann et al} demonstrates how attackers can detect applications running in co-resident virtual machines using deduplication-based side channels. This approach highlights the risks of shared environments in multi-tenant systems\cite{lindemann2018memory}. Remote Memory-Deduplication Attacks extends these techniques to a fully remote setting, where attackers disclose memory contents from a remote server by timing HTTP network requests. This work underscores the far-reaching implications of deduplication-based vulnerabilities\cite{schwarzl2021remote}. Breaking KASLR Using Memory Deduplication in Virtualized Environments expands on these concepts, presenting a memory-sharing-based side-channel attack to break Kernel Address Space Layout Randomization (KASLR) on KPTI-enabled Linux virtual machines\cite{kim2021breaking}. \textit{suzaki et al} discusses how deduplication impacts cryptographic libraries, providing avenues for attackers to leak sensitive data. This emphasizes the dual nature of deduplication as both a performance tool and a security risk\cite{suzaki2013implementation}. Memory Deduplication as a Threat to the Guest OS further illustrates how deduplication mechanisms can reveal the presence of specific applications in co-resident virtual machines, posing a severe threat to isolation\cite{suzaki2011memory}. \textit{bosman et al} introduces advanced memory deduplication attacks, including cross-VM data leakage and sandboxed JavaScript exploits. These attacks highlight the versatile risks associated with deduplication mechanisms\cite{bosman2016dedup}.

\end{itemize}

\section{Hardware-Based Attacks} The hardware layer, while foundational to modern computing, introduces vulnerabilities deeply embedded within the physical architecture of systems. Unlike software-based attacks, which often exploit flaws in program logic or execution, hardware-based side-channel attacks target the fundamental design of hardware components. These attacks exploit unintended behaviors in physical systems, such as memory operations, power fluctuations, or resource contention, exposing the risks inherent in the trade-offs between performance, efficiency, and security. Among the most studied categories are DRAM-based attacks, which exploit vulnerabilities in memory hardware to breach isolation boundaries. The groundbreaking Rowhammer attack revealed how repeatedly activating rows in DRAM could induce bit flips in neighboring rows, compromising data integrity\cite{mutlu2019rowhammer}. Building on this, TRRespass demonstrated how mitigation techniques like Target Row Refresh (TRR) could be bypassed, further exposing DRAM’s fragility \cite{frigo2020trrespass}. These attacks underscore the systemic risks posed by hardware optimizations in modern memory technologies. Beyond memory, the hardware ecosystem includes peripherals and interconnects, which are increasingly exploited in side-channel attacks. For instance, cold boot attacks leverage residual data in memory after a system powers down, bypassing conventional software protections.Shared resources, such as caches and interconnects, represent another critical vulnerability. Techniques like Flush+Reload and Prime+Probe exploit timing discrepancies to infer sensitive data, particularly in multi-tenant environments \cite{gruss2015cache, kocher2020spectr}. More recently, dynamic cache partitioning approaches, \textit{dessouky et al.}, have been proposed to isolate workloads and mitigate these risks \cite{dessouky2020hybcache}.
Physical characteristics of hardware, such as power consumption or electromagnetic emissions, also reveal sensitive data. Attacks like TLBleed exploit timing differences in translation lookaside buffers, while RAMBleed manipulates memory access patterns to leak cryptographic keys \cite{gras2018tlbleed, kwong2020rambleed}. These attacks highlight how physical side channels bypass even the most sophisticated cryptographic defenses. Finally, the rise of parallel computing architectures, such as GPUs, introduces unique vulnerabilities. Attacks like GPUMemory leverage execution timing and resource contention to infer sensitive computations\cite{naghibijouybari2018rendered}. Similarly, shared buses and interconnects, exploited by techniques like DRAMA, reveal the systemic risks of shared hardware resources in virtualized environments\cite{pessl2016drama}.
In the following sections, we delve deeper into these attack types, systematically exploring their mechanisms, impacts, and countermeasures. By understanding these vulnerabilities, we can better appreciate the evolving threat landscape and the need for innovative hardware-level defenses.

\subsection{Memory-Specific Exploitation:}
Memory systems are integral to modern computing, yet they harbor vulnerabilities that attackers can exploit to compromise data integrity and confidentiality. These attacks leverage flaws in DRAM architecture, memory retention, and row buffer management to gain unauthorized access to sensitive information.

\begin{itemize}
    \item \textbf{DRAM-Based Attacks:} Dynamic Random-Access Memory (DRAM) is a prime target for hardware-based attacks. Rowhammer, introduced by \textit{mutlu et al.}, revealed how activating a single row could cause bit flips in adjacent rows \cite{mutlu2019rowhammer}. TRRespass bypassed mitigation mechanisms like Target Row Refresh (TRR), showing the continued risk to DRAM\cite{frigo2020trrespass}. Techniques such as Blacksmith and ZenHammer demonstrate DRAM's ongoing susceptibility \cite{jattke2022blacksmith, jattke2024zenhammer}. Rowhammer.js and Throwhammer extend attacks to web browsers and networks\cite{gruss2016rowhammer, tatar2018throwhammer}. DRAMMER targets mobile platforms, while HammerScope observes power patterns\cite{van2016drammer, cohen2022hammerscope}. A New Approach for Rowhammer Attacks introduces enhanced methods for bit flips\cite{qiao2016new}.

    \item \textbf{Cold Boot Attacks:}
    Cold boot attacks exploit DRAM’s transient data retention to recover sensitive data like encryption keys. Introduced by Halderman et al. (2008), they remain effective even with modern scrambling techniques\cite{halderman2009lest}. Studies like DeepFreeze recover machine learning models, while On Recovering Block Cipher Secret Keys combines cold boot methods with quantum algorithms\cite{halderman2009lest, guo2022don}. Cold Boot Attacks on LUOV and Recovering AES Keys with a Deep Cold Boot Attack expand these methods to cryptographic vulnerabilities\cite{zimerman2021recovering,villanueva2020cold}.Hidden in Snow, Revealed in Thaw revisits these attacks' practicality in modern systems\cite{wetzels2014hidden}.

    \item \textbf{Row Buffer Attacks:}
    Row buffer exploits manipulate DRAM’s optimization mechanisms to create covert channels or leak information. The DRAMA attack exemplifies this by targeting row buffer conflicts]\cite{pessl2016drama}, while Throwhammer enables remote exploitation\cite{tatar2018throwhammer}. Techniques like Flipping Bits in Memory Without Accessing Them and RowPress amplify disturbance errors in DRAM chips\cite{kim2014flipping, luo2023rowpress}. It’s Hammer Time focuses on exploiting Rowhammer vulnerabilities in DRAM-based Physical Unclonable Functions (PUFs)\cite{zeitouni2018s} ChargeCache demonstrates how row access locality can aid attacks\cite{hassan2016chargecache}. The Half-Double attack extends Rowhammer techniques to induce bit flips in adjacent rows\cite{kogler2022half}.
\end{itemize}

\subsection{Physical Analysis Exploitation:}Physical analysis exploitation involves leveraging physical characteristics of hardware to extract sensitive information or induce unintended behavior. By targeting vulnerabilities inherent in hardware properties, these attacks exploit mechanisms like power variations, thermal fluctuations, and electromagnetic radiation to compromise system security. This section delves into Power Analysis Exploitation, Thermal Attacks, and Spectroscopy-Based Exploitation, highlighting their implications across modern systems.
\begin{itemize}
    \item \textbf{Power Analysis Exploitation}
    Power analysis attacks exploit variations in a device's power consumption to infer sensitive information, such as cryptographic keys or operational data. These techniques, including Simple Power Analysis (SPA) and Differential Power Analysis (DPA), target variations in power usage to reveal critical data. Machine learning-based approaches further enhance the adaptability of these methods, allowing attackers to generalize across multiple cryptographic algorithms. For example, Correlation Power Analysis (CPA) effectively extracts private keys from systems like FPGA implementations of CRYSTALS-Dilithium [CRYSTALS-Dilithium][Perin et al. (2024)]. Additionally, innovations like LeakyOhm exploit impedance changes in power distribution networks, underscoring the evolving sophistication of these attacks [LeakyOhm][Arora et al. (2023)]. 

\end{itemize}
